# Supplementary material for: AdaCap: Adaptive Capacity control for Feed-Forward Neural Networks
Source: arXiv:2205.07860 source file (2022-05-09)
Supplement: Supplementary file 1 [file AppendixTableTop10AvgMethod.tex]

\clearpage

\begin{table}[h]
\label{tab:architectureinfos}
\centering
\footnotesize
\begin{tabular}{|l||c|c|c|c|}
\hline
category & method & \RMSE{} & \Rscore{} & avg. running time \\
\hline
\hline
\trainmet{} & \mlrnetselu & $0.4147$ & $0.7710$ & $19.798$ \\
\DNN{} & \regularnetglu & $0.4201$ & $0.7662$ & $9.8911$ \\
\trainmet{} & \mlrnetglu & $0.4206$ & $0.7613$ & $22.355$ \\
\trainmet{} & \mlrnetresblock & $0.4214$ & $0.7667$ & $17.192$ \\
\GBDT{} & \Catboost{} & $0.4221$ & $0.7724$ & $92.518$ \\
\DNN{} & \regularnetstandard & $0.4230$ & $0.7653$ & $4.0581$ \\
\trainmet{} & \mlrnetstandard & $0.4233$ & $0.7635$ & $17.208$ \\
\trainmet{} & \mlrnetfastselu & $0.4245$ & $0.7632$ & $7.6670$ \\
\trainmet{} & \mlrnetbatchresblock & $0.4257$ & $0.7640$ & $194.72$ \\
\DNN{} & \regularnetselu & $0.4260$ & $0.7609$ & $7.1895$ \\
\hline
\end{tabular}
\caption{Average \RMSE{} performance for top $10$ methods }
\end{table}

\begin{table}[h]
\label{tab:architectureinfos}
\centering
\footnotesize
\begin{tabular}{|l||c|c|c|c|}
\hline
category & method & \RMSE{} & \Rscore{} & avg. running time \\
\hline
\hline
\trainmet{} & \mlrnetselu & $0.3934$ & $0.7733$ & $4.5285$ \\
\trainmet{} & \mlrnetfastselu & $0.4015$ & $0.7662$ & $2.3764$ \\
\DNN{} & \regularnetselu & $0.4016$ & $0.7661$ & $3.4039$ \\
\GBDT{} & \Catboost{} & $0.4019$ & $0.7806$ & $38.132$ \\
\trainmet{} & \mlrnetresblock & $0.4029$ & $0.7683$ & $3.5673$ \\
\trainmet{} & \mlrnetbatchresblock & $0.4042$ & $0.7679$ & $214.91$ \\
\DNN{} & \regularnetfastselu & $0.4044$ & $0.7677$ & $2.2407$ \\
\trainmet{} & \mlrnetglu & $0.4049$ & $0.7571$ & $5.8542$ \\
\trainmet{} & \mlrnetstandard & $0.4064$ & $0.7619$ & $3.9111$ \\
\DNN{} & \regularnetglu & $0.4067$ & $0.7632$ & $4.8544$ \\
\hline
\end{tabular}
\caption{Average \RMSE{} performance for top $10$ methods  with $n <= 1000$}
\end{table}

\begin{table}[h]
\label{tab:architectureinfos}
\centering
\footnotesize
\begin{tabular}{|l||c|c|c|c|}
\hline
category & method & \RMSE{} & \Rscore{} & avg. running time \\
\hline
\hline
\trainmet{} & \mlrnetselu & $0.1892$ & $0.9551$ & $20.563$ \\
\trainmet{} & \mlrnetglu & $0.1911$ & $0.9533$ & $22.412$ \\
\DNN{} & \regularnetglu & $0.1976$ & $0.9499$ & $7.3567$ \\
\DNN{} & \regularnetselu & $0.1985$ & $0.9499$ & $5.2767$ \\
\trainmet{} & \mlrnetresblock & $0.1988$ & $0.9503$ & $19.755$ \\
\trainmet{} & \mlrnetstandard & $0.2004$ & $0.9505$ & $19.734$ \\
\trainmet{} & \mlrnetfastselu & $0.2006$ & $0.9501$ & $5.8620$ \\
\trainmet{} & \mlrnetbatchresblock & $0.2032$ & $0.9484$ & $229.29$ \\
\DNN{} & \regularnetstandard & $0.2047$ & $0.9482$ & $4.1063$ \\
\trainmet{} & \mlrnetfast & $0.2065$ & $0.9478$ & $5.0615$ \\
\hline
\end{tabular}
\caption{Average \RMSE{} performance for top $10$ methods  with min \RMSE{} $<= 0.3$}
\end{table}

\begin{table}[h]
\label{tab:architectureinfos}
\centering
\footnotesize
\begin{tabular}{|l||c|c|c|c|}
\hline
category & method & \RMSE{} & \Rscore{} & avg. running time \\
\hline
\hline
\DNN{} & \regularnetglu & $0.4201$ & $0.7662$ & $9.8911$ \\
\GBDT{} & \Catboost{} & $0.4221$ & $0.7724$ & $92.518$ \\
\DNN{} & \regularnetstandard & $0.4230$ & $0.7653$ & $4.0581$ \\
\DNN{} & \regularnetselu & $0.4260$ & $0.7609$ & $7.1895$ \\
\DNN{} & \regularnetresblock & $0.4282$ & $0.7541$ & $18.083$ \\
\DNN{} & \regularnetfast & $0.4312$ & $0.7612$ & $1.5870$ \\
\DNN{} & \regularnetfastselu & $0.4391$ & $0.7507$ & $5.2658$ \\
\RF{} & \RF{} & $0.4421$ & $0.7584$ & $3.6628$ \\
\DNN{} & \regularnetbatchresblock & $0.4436$ & $0.7418$ & $186.81$ \\
\GBDT{} & \XGBoost{} & $0.4528$ & $0.7367$ & $0.8504$ \\
\hline
\end{tabular}
\caption{Average \RMSE{} performance for top $10$ methods excluding \trainmet{} }
\end{table}

\begin{table}[h]
\label{tab:architectureinfos}
\centering
\footnotesize
\begin{tabular}{|l||c|c|c|c|}
\hline
category & method & \RMSE{} & \Rscore{} & avg. running time \\
\hline
\hline
\DNN{} & \regularnetselu & $0.4016$ & $0.7661$ & $3.4039$ \\
\GBDT{} & \Catboost{} & $0.4019$ & $0.7806$ & $38.132$ \\
\DNN{} & \regularnetfastselu & $0.4044$ & $0.7677$ & $2.2407$ \\
\DNN{} & \regularnetglu & $0.4067$ & $0.7632$ & $4.8544$ \\
\DNN{} & \regularnetstandard & $0.4084$ & $0.7632$ & $2.2684$ \\
\DNN{} & \regularnetfast & $0.4127$ & $0.7640$ & $0.9433$ \\
\DNN{} & \regularnetresblock & $0.4193$ & $0.7427$ & $4.2525$ \\
\GBDT{} & \Fastcat & $0.4212$ & $0.7694$ & $0.7658$ \\
\DNN{} & \regularnetbatchresblock & $0.4233$ & $0.7605$ & $191.25$ \\
\GBDT{} & \XGBsklearn{} & $0.4249$ & $0.7526$ & $0.1022$ \\
\hline
\end{tabular}
\caption{Average \RMSE{} performance for top $10$ methods excluding \trainmet{}  with $n <= 1000$}
\end{table}

\begin{table}[h]
\label{tab:architectureinfos}
\centering
\footnotesize
\begin{tabular}{|l||c|c|c|c|}
\hline
category & method & \RMSE{} & \Rscore{} & avg. running time \\
\hline
\hline
\DNN{} & \regularnetglu & $0.1961$ & $0.9506$ & $7.3970$ \\
\DNN{} & \regularnetselu & $0.1971$ & $0.9505$ & $5.3057$ \\
\DNN{} & \regularnetstandard & $0.2031$ & $0.9490$ & $4.1239$ \\
\DNN{} & \regularnetresblock & $0.2076$ & $0.9471$ & $20.826$ \\
\DNN{} & \regularnetfast & $0.2119$ & $0.9454$ & $1.6239$ \\
\DNN{} & \regularnetfastselu & $0.2136$ & $0.9436$ & $2.9069$ \\
\GBDT{} & \Catboost{} & $0.2217$ & $0.9387$ & $71.093$ \\
\RF{} & \XRF{} & $0.2320$ & $0.9362$ & $1.4362$ \\
\DNN{} & \regularnetbatchresblock & $0.2409$ & $0.9116$ & $219.43$ \\
\GBDT{} & \XGBoost{} & $0.2433$ & $0.9257$ & $0.7540$ \\
\hline
\end{tabular}
\caption{Average \RMSE{} performance for top $10$ methods excluding \trainmet{}  with min \RMSE{} $<= 0.3$}
\end{table}

\begin{table}[h]
\label{tab:architectureinfos}
\centering
\footnotesize
\begin{tabular}{|l||c|c|c|c|}
\hline
category & method & \ERR{} & \AUC{} & avg. running time \\
\hline
\hline
\GBDT{} & \Catboost{} & $0.1428$ & $0.8952$ & $189.63$ \\
\RF{} & \RF{} & $0.1500$ & $0.8916$ & $0.8067$ \\
\GBDT{} & \Fastcat & $0.1512$ & $0.8840$ & $1.7523$ \\
\GBDT{} & \lightgbm{} & $0.1524$ & $0.8804$ & $0.3372$ \\
\GBDT{} & \XGBoost{} & $0.1552$ & $0.8819$ & $2.5522$ \\
\RF{} & \XRF{} & $0.1559$ & $0.8827$ & $0.6778$ \\
\GBDT{} & \XGBsklearn{} & $0.1591$ & $0.8807$ & $2.9999$ \\
\DNN{} & \regularnetfast & $0.1666$ & $0.8705$ & $1.5031$ \\
\DNN{} & \regularnetselu & $0.1667$ & $0.8716$ & $10.460$ \\
\trainmet{} & \mlrnetfast & $0.1670$ & $0.8716$ & $3.1070$ \\
\hline
\end{tabular}
\caption{Average \ERR{} performance for top $10$ methods }
\end{table}

\begin{table}[h]
\label{tab:architectureinfos}
\centering
\footnotesize
\begin{tabular}{|l||c|c|c|c|}
\hline
category & method & \ERR{} & \AUC{} & avg. running time \\
\hline
\hline
\GBDT{} & \Catboost{} & $0.1344$ & $0.8948$ & $64.400$ \\
\GBDT{} & \Fastcat & $0.1397$ & $0.8853$ & $0.9808$ \\
\RF{} & \RF{} & $0.1408$ & $0.8928$ & $0.1496$ \\
\GBDT{} & \lightgbm{} & $0.1454$ & $0.8772$ & $0.0355$ \\
\GBDT{} & \XGBoost{} & $0.1472$ & $0.8812$ & $0.0893$ \\
\RF{} & \XRF{} & $0.1486$ & $0.8811$ & $0.1256$ \\
\GBDT{} & \XGBsklearn{} & $0.1524$ & $0.8792$ & $0.1090$ \\
\GLM{} & \Enet{} & $0.1561$ & $0.8647$ & $1.9172$ \\
\trainmet{} & \mlrnetfast & $0.1566$ & $0.8727$ & $1.7508$ \\
\DNN{} & \regularnetfast & $0.1567$ & $0.8698$ & $1.1283$ \\
\hline
\end{tabular}
\caption{Average \ERR{} performance for top $10$ methods  with $n <= 1000$}
\end{table}

\begin{table}[h]
\label{tab:architectureinfos}
\centering
\footnotesize
\begin{tabular}{|l||c|c|c|c|}
\hline
category & method & \ERR{} & \AUC{} & avg. running time \\
\hline
\hline
\GBDT{} & \Catboost{} & $0.1428$ & $0.8952$ & $189.63$ \\
\RF{} & \RF{} & $0.1500$ & $0.8916$ & $0.8067$ \\
\GBDT{} & \Fastcat & $0.1512$ & $0.8840$ & $1.7523$ \\
\GBDT{} & \lightgbm{} & $0.1524$ & $0.8804$ & $0.3372$ \\
\GBDT{} & \XGBoost{} & $0.1552$ & $0.8819$ & $2.5522$ \\
\RF{} & \XRF{} & $0.1559$ & $0.8827$ & $0.6778$ \\
\GBDT{} & \XGBsklearn{} & $0.1591$ & $0.8807$ & $2.9999$ \\
\DNN{} & \regularnetfast & $0.1666$ & $0.8705$ & $1.5031$ \\
\DNN{} & \regularnetselu & $0.1667$ & $0.8716$ & $10.460$ \\
\trainmet{} & \mlrnetfast & $0.1670$ & $0.8716$ & $3.1070$ \\
\hline
\end{tabular}
\caption{Average \ERR{} performance for top $10$ methods  with min \ERR{} $<= 0.3$}
\end{table}

\begin{table}[h]
\label{tab:architectureinfos}
\centering
\footnotesize
\begin{tabular}{|l||c|c|c|c|}
\hline
category & method & \ERR{} & \AUC{} & avg. running time \\
\hline
\hline
\GBDT{} & \Catboost{} & $0.1428$ & $0.8952$ & $189.63$ \\
\RF{} & \RF{} & $0.1500$ & $0.8916$ & $0.8067$ \\
\GBDT{} & \Fastcat & $0.1512$ & $0.8840$ & $1.7523$ \\
\GBDT{} & \lightgbm{} & $0.1524$ & $0.8804$ & $0.3372$ \\
\GBDT{} & \XGBoost{} & $0.1552$ & $0.8819$ & $2.5522$ \\
\RF{} & \XRF{} & $0.1559$ & $0.8827$ & $0.6778$ \\
\GBDT{} & \XGBsklearn{} & $0.1591$ & $0.8807$ & $2.9999$ \\
\DNN{} & \regularnetfast & $0.1666$ & $0.8705$ & $1.5031$ \\
\DNN{} & \regularnetselu & $0.1667$ & $0.8716$ & $10.460$ \\
\DNN{} & \regularnetstandard & $0.1688$ & $0.8703$ & $3.8363$ \\
\hline
\end{tabular}
\caption{Average \ERR{} performance for top $10$ methods excluding \trainmet{} }
\end{table}

\begin{table}[h]
\label{tab:architectureinfos}
\centering
\footnotesize
\begin{tabular}{|l||c|c|c|c|}
\hline
category & method & \ERR{} & \AUC{} & avg. running time \\
\hline
\hline
\GBDT{} & \Catboost{} & $0.1344$ & $0.8948$ & $64.400$ \\
\GBDT{} & \Fastcat & $0.1397$ & $0.8853$ & $0.9808$ \\
\RF{} & \RF{} & $0.1408$ & $0.8928$ & $0.1496$ \\
\GBDT{} & \lightgbm{} & $0.1454$ & $0.8772$ & $0.0355$ \\
\GBDT{} & \XGBoost{} & $0.1472$ & $0.8812$ & $0.0893$ \\
\RF{} & \XRF{} & $0.1486$ & $0.8811$ & $0.1256$ \\
\GBDT{} & \XGBsklearn{} & $0.1524$ & $0.8792$ & $0.1090$ \\
\GLM{} & \Enet{} & $0.1561$ & $0.8647$ & $1.9172$ \\
\DNN{} & \regularnetfast & $0.1567$ & $0.8698$ & $1.1283$ \\
\DNN{} & \regularnetselu & $0.1600$ & $0.8704$ & $7.5148$ \\
\hline
\end{tabular}
\caption{Average \ERR{} performance for top $10$ methods excluding \trainmet{}  with $n <= 1000$}
\end{table}

\begin{table}[h]
\label{tab:architectureinfos}
\centering
\footnotesize
\begin{tabular}{|l||c|c|c|c|}
\hline
category & method & \ERR{} & \AUC{} & avg. running time \\
\hline
\hline
\GBDT{} & \Catboost{} & $0.1428$ & $0.8952$ & $189.63$ \\
\RF{} & \RF{} & $0.1500$ & $0.8916$ & $0.8067$ \\
\GBDT{} & \Fastcat & $0.1512$ & $0.8840$ & $1.7523$ \\
\GBDT{} & \lightgbm{} & $0.1524$ & $0.8804$ & $0.3372$ \\
\GBDT{} & \XGBoost{} & $0.1552$ & $0.8819$ & $2.5522$ \\
\RF{} & \XRF{} & $0.1559$ & $0.8827$ & $0.6778$ \\
\GBDT{} & \XGBsklearn{} & $0.1591$ & $0.8807$ & $2.9999$ \\
\DNN{} & \regularnetfast & $0.1666$ & $0.8705$ & $1.5031$ \\
\DNN{} & \regularnetselu & $0.1667$ & $0.8716$ & $10.460$ \\
\DNN{} & \regularnetstandard & $0.1688$ & $0.8703$ & $3.8363$ \\
\hline
\end{tabular}
\caption{Average \ERR{} performance for top $10$ methods excluding \trainmet{}  with min \ERR{} $<= 0.3$}
\end{table}
