# Supplementary material for: AdaCap: Adaptive Capacity control for Feed-Forward Neural Networks
Source: arXiv:2205.07860 source file (2022-05-09)
Supplement: Supplementary file 2 [file AppendixTableTop1CountCateg.tex]

\clearpage

\begin{table}[h]
\centering
\footnotesize
\begin{tabular}{|l||c|c|c|}
\hline
category & \AUC{} and \Rscore{} & \%WIN & \# Datasets splits \\
\hline
\hline
\GBDT{} & $205$ & $46.59$ & $440$ \\
\DNN{} & $126$ & $28.63$ & $440$ \\
\RF{} & $72$ & $16.36$ & $440$ \\
\GLM{} & $20$ & $4.545$ & $440$ \\
\SVM{} & $13$ & $2.954$ & $440$ \\
\MARS{} & $4$ & $0.909$ & $440$ \\
\hline
\end{tabular}
\caption{category top1 count excluding \trainmet{} for \AUC{} and \Rscore{}}
\end{table}

\begin{table}[h]
\centering
\footnotesize
\begin{tabular}{|l||c|c|c|}
\hline
category & \AUC{} and \Rscore{} & \%WIN & \# Datasets splits \\
\hline
\hline
\GBDT{} & $130$ & $46.42$ & $280$ \\
\DNN{} & $86$ & $30.71$ & $280$ \\
\RF{} & $32$ & $11.42$ & $280$ \\
\GLM{} & $19$ & $6.785$ & $280$ \\
\SVM{} & $9$ & $3.214$ & $280$ \\
\MARS{} & $4$ & $1.428$ & $280$ \\
\hline
\end{tabular}
\caption{category top1 count excluding \trainmet{} for \AUC{} and \Rscore{} with $n <= 1000$}
\end{table}

\begin{table}[h]
\centering
\footnotesize
\begin{tabular}{|l||c|c|c|}
\hline
category & \AUC{} and \Rscore{} & \%WIN & \# Datasets splits \\
\hline
\hline
\GBDT{} & $194$ & $44.09$ & $440$ \\
\trainmet{} & $79$ & $17.95$ & $440$ \\
\DNN{} & $69$ & $15.68$ & $440$ \\
\RF{} & $68$ & $15.45$ & $440$ \\
\GLM{} & $17$ & $3.863$ & $440$ \\
\SVM{} & $11$ & $2.5$ & $440$ \\
\MARS{} & $2$ & $0.454$ & $440$ \\
\hline
\end{tabular}
\caption{category top1 count for \AUC{} and \Rscore{}}
\end{table}

\begin{table}[h]
\centering
\footnotesize
\begin{tabular}{|l||c|c|c|}
\hline
category & \AUC{} and \Rscore{} & \%WIN & \# Datasets splits \\
\hline
\hline
\GBDT{} & $119$ & $42.5$ & $280$ \\
\trainmet{} & $57$ & $20.35$ & $280$ \\
\DNN{} & $50$ & $17.85$ & $280$ \\
\RF{} & $28$ & $10.0$ & $280$ \\
\GLM{} & $16$ & $5.714$ & $280$ \\
\SVM{} & $8$ & $2.857$ & $280$ \\
\MARS{} & $2$ & $0.714$ & $280$ \\
\hline
\end{tabular}
\caption{category top1 count for \AUC{} and \Rscore{} with $n <= 1000$}
\end{table}

\begin{table}[h]
\centering
\footnotesize
\begin{tabular}{|l||c|c|c|}
\hline
category & \ERR{} and \RMSE{} & \%WIN & \# Datasets splits \\
\hline
\hline
\GBDT{} & $221$ & $50.22$ & $440$ \\
\DNN{} & $108$ & $24.54$ & $440$ \\
\RF{} & $65$ & $14.77$ & $440$ \\
\GLM{} & $25$ & $5.681$ & $440$ \\
\SVM{} & $13$ & $2.954$ & $440$ \\
\MARS{} & $4$ & $0.909$ & $440$ \\
\CART{} & $4$ & $0.909$ & $440$ \\
\hline
\end{tabular}
\caption{category top1 count excluding \trainmet{} for \ERR{} and \RMSE{}}
\end{table}

\begin{table}[h]
\centering
\footnotesize
\begin{tabular}{|l||c|c|c|}
\hline
category & \ERR{} and \RMSE{} & \%WIN & \# Datasets splits \\
\hline
\hline
\GBDT{} & $145$ & $51.78$ & $280$ \\
\DNN{} & $68$ & $24.28$ & $280$ \\
\RF{} & $26$ & $9.285$ & $280$ \\
\GLM{} & $24$ & $8.571$ & $280$ \\
\SVM{} & $9$ & $3.214$ & $280$ \\
\MARS{} & $4$ & $1.428$ & $280$ \\
\CART{} & $4$ & $1.428$ & $280$ \\
\hline
\end{tabular}
\caption{category top1 count excluding \trainmet{} for \ERR{} and \RMSE{} with $n <= 1000$}
\end{table}

\begin{table}[h]
\centering
\footnotesize
\begin{tabular}{|l||c|c|c|}
\hline
category & \ERR{} and \RMSE{} & \%WIN & \# Datasets splits \\
\hline
\hline
\GBDT{} & $138$ & $55.87$ & $247$ \\
\DNN{} & $62$ & $25.10$ & $247$ \\
\RF{} & $29$ & $11.74$ & $247$ \\
\GLM{} & $14$ & $5.668$ & $247$ \\
\CART{} & $4$ & $1.619$ & $247$ \\
\hline
\end{tabular}
\caption{category top1 count excluding \trainmet{} for \ERR{} and \RMSE{} with min \ERR{} and \RMSE{} $<= 0.25$}
\end{table}

\begin{table}[h]
\centering
\footnotesize
\begin{tabular}{|l||c|c|c|}
\hline
category & \ERR{} and \RMSE{} & \%WIN & \# Datasets splits \\
\hline
\hline
\GBDT{} & $211$ & $47.95$ & $440$ \\
\trainmet{} & $71$ & $16.13$ & $440$ \\
\RF{} & $62$ & $14.09$ & $440$ \\
\DNN{} & $54$ & $12.27$ & $440$ \\
\GLM{} & $25$ & $5.681$ & $440$ \\
\SVM{} & $11$ & $2.5$ & $440$ \\
\CART{} & $4$ & $0.909$ & $440$ \\
\MARS{} & $2$ & $0.454$ & $440$ \\
\hline
\end{tabular}
\caption{category top1 count for \ERR{} and \RMSE{}}
\end{table}

\begin{table}[h]
\centering
\footnotesize
\begin{tabular}{|l||c|c|c|}
\hline
category & \ERR{} and \RMSE{} & \%WIN & \# Datasets splits \\
\hline
\hline
\GBDT{} & $135$ & $48.21$ & $280$ \\
\trainmet{} & $49$ & $17.5$ & $280$ \\
\DNN{} & $35$ & $12.5$ & $280$ \\
\GLM{} & $24$ & $8.571$ & $280$ \\
\RF{} & $23$ & $8.214$ & $280$ \\
\SVM{} & $8$ & $2.857$ & $280$ \\
\CART{} & $4$ & $1.428$ & $280$ \\
\MARS{} & $2$ & $0.714$ & $280$ \\
\hline
\end{tabular}
\caption{category top1 count for \ERR{} and \RMSE{} with $n <= 1000$}
\end{table}

\begin{table}[h]
\centering
\footnotesize
\begin{tabular}{|l||c|c|c|}
\hline
category & \ERR{} and \RMSE{} & \%WIN & \# Datasets splits \\
\hline
\hline
\GBDT{} & $129$ & $51.80$ & $249$ \\
\trainmet{} & $49$ & $19.67$ & $249$ \\
\RF{} & $27$ & $10.84$ & $249$ \\
\DNN{} & $26$ & $10.44$ & $249$ \\
\GLM{} & $14$ & $5.622$ & $249$ \\
\CART{} & $4$ & $1.606$ & $249$ \\
\hline
\end{tabular}
\caption{category top1 count for \ERR{} and \RMSE{} with min \ERR{} and \RMSE{} $<= 0.25$}
\end{table}

\begin{table}[h]
\centering
\footnotesize
\begin{tabular}{|l||c|c|c|}
\hline
category & \Rscore{} & \%WIN & \# Datasets splits \\
\hline
\hline
\GBDT{} & $97$ & $37.30$ & $260$ \\
\DNN{} & $88$ & $33.84$ & $260$ \\
\RF{} & $47$ & $18.07$ & $260$ \\
\SVM{} & $13$ & $5.0$ & $260$ \\
\GLM{} & $11$ & $4.230$ & $260$ \\
\MARS{} & $4$ & $1.538$ & $260$ \\
\hline
\end{tabular}
\caption{category top1 count excluding \trainmet{} for \Rscore{}}
\end{table}

\begin{table}[h]
\centering
\footnotesize
\begin{tabular}{|l||c|c|c|}
\hline
category & \Rscore{} & \%WIN & \# Datasets splits \\
\hline
\hline
\GBDT{} & $64$ & $42.66$ & $150$ \\
\DNN{} & $49$ & $32.66$ & $150$ \\
\RF{} & $14$ & $9.333$ & $150$ \\
\GLM{} & $10$ & $6.666$ & $150$ \\
\SVM{} & $9$ & $6.0$ & $150$ \\
\MARS{} & $4$ & $2.666$ & $150$ \\
\hline
\end{tabular}
\caption{category top1 count excluding \trainmet{} for \Rscore{} with $n <= 1000$}
\end{table}

\begin{table}[h]
\centering
\footnotesize
\begin{tabular}{|l||c|c|c|}
\hline
category & \Rscore{} & \%WIN & \# Datasets splits \\
\hline
\hline
\GBDT{} & $91$ & $35.0$ & $260$ \\
\trainmet{} & $59$ & $22.69$ & $260$ \\
\RF{} & $46$ & $17.69$ & $260$ \\
\DNN{} & $40$ & $15.38$ & $260$ \\
\GLM{} & $11$ & $4.230$ & $260$ \\
\SVM{} & $11$ & $4.230$ & $260$ \\
\MARS{} & $2$ & $0.769$ & $260$ \\
\hline
\end{tabular}
\caption{category top1 count for \Rscore{}}
\end{table}

\begin{table}[h]
\centering
\footnotesize
\begin{tabular}{|l||c|c|c|}
\hline
category & \Rscore{} & \%WIN & \# Datasets splits \\
\hline
\hline
\GBDT{} & $58$ & $38.66$ & $150$ \\
\trainmet{} & $37$ & $24.66$ & $150$ \\
\DNN{} & $22$ & $14.66$ & $150$ \\
\RF{} & $13$ & $8.666$ & $150$ \\
\GLM{} & $10$ & $6.666$ & $150$ \\
\SVM{} & $8$ & $5.333$ & $150$ \\
\MARS{} & $2$ & $1.333$ & $150$ \\
\hline
\end{tabular}
\caption{category top1 count for \Rscore{} with $n <= 1000$}
\end{table}

\begin{table}[h]
\centering
\footnotesize
\begin{tabular}{|l||c|c|c|}
\hline
category & \RMSE{} & \%WIN & \# Datasets splits \\
\hline
\hline
\GBDT{} & $97$ & $37.30$ & $260$ \\
\DNN{} & $88$ & $33.84$ & $260$ \\
\RF{} & $47$ & $18.07$ & $260$ \\
\SVM{} & $13$ & $5.0$ & $260$ \\
\GLM{} & $11$ & $4.230$ & $260$ \\
\MARS{} & $4$ & $1.538$ & $260$ \\
\hline
\end{tabular}
\caption{category top1 count excluding \trainmet{} for \RMSE{}}
\end{table}

\begin{table}[h]
\centering
\footnotesize
\begin{tabular}{|l||c|c|c|}
\hline
category & \RMSE{} & \%WIN & \# Datasets splits \\
\hline
\hline
\GBDT{} & $64$ & $42.66$ & $150$ \\
\DNN{} & $49$ & $32.66$ & $150$ \\
\RF{} & $14$ & $9.333$ & $150$ \\
\GLM{} & $10$ & $6.666$ & $150$ \\
\SVM{} & $9$ & $6.0$ & $150$ \\
\MARS{} & $4$ & $2.666$ & $150$ \\
\hline
\end{tabular}
\caption{category top1 count excluding \trainmet{} for \RMSE{} with $n <= 1000$}
\end{table}

\begin{table}[h]
\centering
\footnotesize
\begin{tabular}{|l||c|c|c|}
\hline
category & \RMSE{} & \%WIN & \# Datasets splits \\
\hline
\hline
\DNN{} & $44$ & $55.00$ & $80$ \\
\GBDT{} & $24$ & $30.0$ & $80$ \\
\RF{} & $12$ & $15.0$ & $80$ \\
\hline
\end{tabular}
\caption{category top1 count excluding \trainmet{} for \RMSE{} with min \RMSE{} $<= 0.25$}
\end{table}

\begin{table}[h]
\centering
\footnotesize
\begin{tabular}{|l||c|c|c|}
\hline
category & \RMSE{} & \%WIN & \# Datasets splits \\
\hline
\hline
\GBDT{} & $91$ & $35.0$ & $260$ \\
\trainmet{} & $59$ & $22.69$ & $260$ \\
\RF{} & $46$ & $17.69$ & $260$ \\
\DNN{} & $40$ & $15.38$ & $260$ \\
\GLM{} & $11$ & $4.230$ & $260$ \\
\SVM{} & $11$ & $4.230$ & $260$ \\
\MARS{} & $2$ & $0.769$ & $260$ \\
\hline
\end{tabular}
\caption{category top1 count for \RMSE{}}
\end{table}

\begin{table}[h]
\centering
\footnotesize
\begin{tabular}{|l||c|c|c|}
\hline
category & \RMSE{} & \%WIN & \# Datasets splits \\
\hline
\hline
\GBDT{} & $58$ & $38.66$ & $150$ \\
\trainmet{} & $37$ & $24.66$ & $150$ \\
\DNN{} & $22$ & $14.66$ & $150$ \\
\RF{} & $13$ & $8.666$ & $150$ \\
\GLM{} & $10$ & $6.666$ & $150$ \\
\SVM{} & $8$ & $5.333$ & $150$ \\
\MARS{} & $2$ & $1.333$ & $150$ \\
\hline
\end{tabular}
\caption{category top1 count for \RMSE{} with $n <= 1000$}
\end{table}

\begin{table}[h]
\centering
\footnotesize
\begin{tabular}{|l||c|c|c|}
\hline
category & \RMSE{} & \%WIN & \# Datasets splits \\
\hline
\hline
\trainmet{} & $37$ & $45.67$ & $81$ \\
\GBDT{} & $19$ & $23.45$ & $81$ \\
\DNN{} & $13$ & $16.04$ & $81$ \\
\RF{} & $12$ & $14.81$ & $81$ \\
\hline
\end{tabular}
\caption{category top1 count for \RMSE{} with min \RMSE{} $<= 0.25$}
\end{table}

\begin{table}[h]
\centering
\footnotesize
\begin{tabular}{|l||c|c|c|}
\hline
category & \AUC{} & \%WIN & \# Datasets splits \\
\hline
\hline
\GBDT{} & $108$ & $60.0$ & $180$ \\
\DNN{} & $38$ & $21.11$ & $180$ \\
\RF{} & $25$ & $13.88$ & $180$ \\
\GLM{} & $9$ & $5.0$ & $180$ \\
\hline
\end{tabular}
\caption{category top1 count excluding \trainmet{} for \AUC{}}
\end{table}

\begin{table}[h]
\centering
\footnotesize
\begin{tabular}{|l||c|c|c|}
\hline
category & \AUC{} & \%WIN & \# Datasets splits \\
\hline
\hline
\GBDT{} & $66$ & $50.76$ & $130$ \\
\DNN{} & $37$ & $28.46$ & $130$ \\
\RF{} & $18$ & $13.84$ & $130$ \\
\GLM{} & $9$ & $6.923$ & $130$ \\
\hline
\end{tabular}
\caption{category top1 count excluding \trainmet{} for \AUC{} with $n <= 1000$}
\end{table}

\begin{table}[h]
\centering
\footnotesize
\begin{tabular}{|l||c|c|c|}
\hline
category & \AUC{} & \%WIN & \# Datasets splits \\
\hline
\hline
\GBDT{} & $103$ & $57.22$ & $180$ \\
\DNN{} & $29$ & $16.11$ & $180$ \\
\RF{} & $22$ & $12.22$ & $180$ \\
\trainmet{} & $20$ & $11.11$ & $180$ \\
\GLM{} & $6$ & $3.333$ & $180$ \\
\hline
\end{tabular}
\caption{category top1 count for \AUC{}}
\end{table}

\begin{table}[h]
\centering
\footnotesize
\begin{tabular}{|l||c|c|c|}
\hline
category & \AUC{} & \%WIN & \# Datasets splits \\
\hline
\hline
\GBDT{} & $61$ & $46.92$ & $130$ \\
\DNN{} & $28$ & $21.53$ & $130$ \\
\trainmet{} & $20$ & $15.38$ & $130$ \\
\RF{} & $15$ & $11.53$ & $130$ \\
\GLM{} & $6$ & $4.615$ & $130$ \\
\hline
\end{tabular}
\caption{category top1 count for \AUC{} with $n <= 1000$}
\end{table}

\begin{table}[h]
\centering
\footnotesize
\begin{tabular}{|l||c|c|c|}
\hline
category & \ERR{} & \%WIN & \# Datasets splits \\
\hline
\hline
\GBDT{} & $124$ & $68.88$ & $180$ \\
\DNN{} & $20$ & $11.11$ & $180$ \\
\RF{} & $18$ & $10.0$ & $180$ \\
\GLM{} & $14$ & $7.777$ & $180$ \\
\CART{} & $4$ & $2.222$ & $180$ \\
\hline
\end{tabular}
\caption{category top1 count excluding \trainmet{} for \ERR{}}
\end{table}

\begin{table}[h]
\centering
\footnotesize
\begin{tabular}{|l||c|c|c|}
\hline
category & \ERR{} & \%WIN & \# Datasets splits \\
\hline
\hline
\GBDT{} & $81$ & $62.30$ & $130$ \\
\DNN{} & $19$ & $14.61$ & $130$ \\
\GLM{} & $14$ & $10.76$ & $130$ \\
\RF{} & $12$ & $9.230$ & $130$ \\
\CART{} & $4$ & $3.076$ & $130$ \\
\hline
\end{tabular}
\caption{category top1 count excluding \trainmet{} for \ERR{} with $n <= 1000$}
\end{table}

\begin{table}[h]
\centering
\footnotesize
\begin{tabular}{|l||c|c|c|}
\hline
category & \ERR{} & \%WIN & \# Datasets splits \\
\hline
\hline
\GBDT{} & $114$ & $68.26$ & $167$ \\
\DNN{} & $18$ & $10.77$ & $167$ \\
\RF{} & $17$ & $10.17$ & $167$ \\
\GLM{} & $14$ & $8.383$ & $167$ \\
\CART{} & $4$ & $2.395$ & $167$ \\
\hline
\end{tabular}
\caption{category top1 count excluding \trainmet{} for \ERR{} with min \ERR{} $<= 0.25$}
\end{table}

\begin{table}[h]
\centering
\footnotesize
\begin{tabular}{|l||c|c|c|}
\hline
category & \ERR{} & \%WIN & \# Datasets splits \\
\hline
\hline
\GBDT{} & $120$ & $66.66$ & $180$ \\
\RF{} & $16$ & $8.888$ & $180$ \\
\GLM{} & $14$ & $7.777$ & $180$ \\
\DNN{} & $14$ & $7.777$ & $180$ \\
\trainmet{} & $12$ & $6.666$ & $180$ \\
\CART{} & $4$ & $2.222$ & $180$ \\
\hline
\end{tabular}
\caption{category top1 count for \ERR{}}
\end{table}

\begin{table}[h]
\centering
\footnotesize
\begin{tabular}{|l||c|c|c|}
\hline
category & \ERR{} & \%WIN & \# Datasets splits \\
\hline
\hline
\GBDT{} & $77$ & $59.23$ & $130$ \\
\GLM{} & $14$ & $10.76$ & $130$ \\
\DNN{} & $13$ & $10.0$ & $130$ \\
\trainmet{} & $12$ & $9.230$ & $130$ \\
\RF{} & $10$ & $7.692$ & $130$ \\
\CART{} & $4$ & $3.076$ & $130$ \\
\hline
\end{tabular}
\caption{category top1 count for \ERR{} with $n <= 1000$}
\end{table}

\begin{table}[h]
\centering
\footnotesize
\begin{tabular}{|l||c|c|c|}
\hline
category & \ERR{} & \%WIN & \# Datasets splits \\
\hline
\hline
\GBDT{} & $110$ & $65.47$ & $168$ \\
\RF{} & $15$ & $8.928$ & $168$ \\
\GLM{} & $14$ & $8.333$ & $168$ \\
\DNN{} & $13$ & $7.738$ & $168$ \\
\trainmet{} & $12$ & $7.142$ & $168$ \\
\CART{} & $4$ & $2.380$ & $168$ \\
\hline
\end{tabular}
\caption{category top1 count for \ERR{} with min \ERR{} $<= 0.25$}
\end{table}
