# Supplementary material for: AdaCap: Adaptive Capacity control for Feed-Forward Neural Networks
Source: arXiv:2205.07860 source file (2022-05-09)
Supplement: Supplementary file 3 [file AppendixTableTop1CountMethod.tex]

\begin{table}[h]
\centering
\footnotesize
\begin{tabular}{|l||c|c|c|}
\hline
method & \AUC{} and \Rscore{} & \%WIN & \# Datasets splits \\
\hline
\hline
\Catboost{} & $101$ & $22.95$ & $440$ \\
\XRF{} & $43$ & $9.772$ & $440$ \\
\XGBsklearn{} & $38$ & $8.636$ & $440$ \\
\regularnetselu & $29$ & $6.590$ & $440$ \\
\RF{} & $29$ & $6.590$ & $440$ \\
\Fastcat & $27$ & $6.136$ & $440$ \\
\XGBoost{} & $21$ & $4.772$ & $440$ \\
\regularnetfastselu & $21$ & $4.772$ & $440$ \\
\regularnetglu & $20$ & $4.545$ & $440$ \\
\regularnetstandard & $16$ & $3.636$ & $440$ \\
\lightgbm{} & $15$ & $3.409$ & $440$ \\
\regularnetbatchstandard & $12$ & $2.727$ & $440$ \\
\regularnetbatchresblock & $12$ & $2.727$ & $440$ \\
\regularnetresblock & $11$ & $2.5$ & $440$ \\
\Kernel{} & $7$ & $1.590$ & $440$ \\
\Enet{} & $7$ & $1.590$ & $440$ \\
\LAS{} & $7$ & $1.590$ & $440$ \\
\Ridge{} & $6$ & $1.363$ & $440$ \\
\NuSVM{} & $6$ & $1.363$ & $440$ \\
\regularnetfast & $5$ & $1.136$ & $440$ \\
\MARS{} & $4$ & $0.909$ & $440$ \\
\Adaboost{} & $3$ & $0.681$ & $440$ \\
\hline
\end{tabular}
\caption{method top1 count excluding \trainmet{} for \AUC{} and \Rscore{}}
\end{table}

\begin{table}[h]
\centering
\footnotesize
\begin{tabular}{|l||c|c|c|}
\hline
method & \AUC{} and \Rscore{} & \%WIN & \# Datasets splits \\
\hline
\hline
\Catboost{} & $59$ & $21.07$ & $280$ \\
\XGBsklearn{} & $27$ & $9.642$ & $280$ \\
\regularnetselu & $26$ & $9.285$ & $280$ \\
\Fastcat & $17$ & $6.071$ & $280$ \\
\XRF{} & $16$ & $5.714$ & $280$ \\
\RF{} & $16$ & $5.714$ & $280$ \\
\XGBoost{} & $14$ & $5.0$ & $280$ \\
\regularnetfastselu & $13$ & $4.642$ & $280$ \\
\regularnetstandard & $13$ & $4.642$ & $280$ \\
\regularnetglu & $12$ & $4.285$ & $280$ \\
\lightgbm{} & $10$ & $3.571$ & $280$ \\
\regularnetbatchresblock & $8$ & $2.857$ & $280$ \\
\LAS{} & $7$ & $2.5$ & $280$ \\
\Enet{} & $7$ & $2.5$ & $280$ \\
\Ridge{} & $5$ & $1.785$ & $280$ \\
\NuSVM{} & $5$ & $1.785$ & $280$ \\
\regularnetfast & $5$ & $1.785$ & $280$ \\
\regularnetresblock & $5$ & $1.785$ & $280$ \\
\regularnetbatchstandard & $4$ & $1.428$ & $280$ \\
\MARS{} & $4$ & $1.428$ & $280$ \\
\Kernel{} & $4$ & $1.428$ & $280$ \\
\Adaboost{} & $3$ & $1.071$ & $280$ \\
\hline
\end{tabular}
\caption{method top1 count excluding \trainmet{} for \AUC{} and \Rscore{} with $n <= 1000$}
\end{table}

\begin{table}[h]
\centering
\footnotesize
\begin{tabular}{|l||c|c|c|}
\hline
method & \AUC{} and \Rscore{} & \%WIN & \# Datasets splits \\
\hline
\hline
\Catboost{} & $94$ & $21.36$ & $440$ \\
\XRF{} & $41$ & $9.318$ & $440$ \\
\XGBsklearn{} & $37$ & $8.409$ & $440$ \\
\mlrnetglu & $30$ & $6.818$ & $440$ \\
\Fastcat & $27$ & $6.136$ & $440$ \\
\RF{} & $27$ & $6.136$ & $440$ \\
\XGBoost{} & $20$ & $4.545$ & $440$ \\
\regularnetselu & $16$ & $3.636$ & $440$ \\
\lightgbm{} & $14$ & $3.181$ & $440$ \\
\mlrnetselu & $12$ & $2.727$ & $440$ \\
\regularnetglu & $11$ & $2.5$ & $440$ \\
\regularnetstandard & $10$ & $2.272$ & $440$ \\
\mlrnetstandard & $10$ & $2.272$ & $440$ \\
\mlrnetfastselu & $9$ & $2.045$ & $440$ \\
\regularnetfastselu & $9$ & $2.045$ & $440$ \\
\regularnetbatchresblock & $8$ & $1.818$ & $440$ \\
\regularnetresblock & $8$ & $1.818$ & $440$ \\
\Enet{} & $7$ & $1.590$ & $440$ \\
\mlrnetfast & $6$ & $1.363$ & $440$ \\
\mlrnetbatchresblock & $6$ & $1.363$ & $440$ \\
\Kernel{} & $6$ & $1.363$ & $440$ \\
\mlrnetresblock & $5$ & $1.136$ & $440$ \\
\Ridge{} & $5$ & $1.136$ & $440$ \\
\regularnetbatchstandard & $5$ & $1.136$ & $440$ \\
\NuSVM{} & $5$ & $1.136$ & $440$ \\
\LAS{} & $5$ & $1.136$ & $440$ \\
\regularnetfast & $2$ & $0.454$ & $440$ \\
\Adaboost{} & $2$ & $0.454$ & $440$ \\
\MARS{} & $2$ & $0.454$ & $440$ \\
\mlrnetbatchstandard & $1$ & $0.227$ & $440$ \\
\hline
\end{tabular}
\caption{method top1 count for \AUC{} and \Rscore{}}
\end{table}

\begin{table}[h]
\centering
\footnotesize
\begin{tabular}{|l||c|c|c|}
\hline
method & \AUC{} and \Rscore{} & \%WIN & \# Datasets splits \\
\hline
\hline
\Catboost{} & $52$ & $18.57$ & $280$ \\
\XGBsklearn{} & $26$ & $9.285$ & $280$ \\
\mlrnetglu & $18$ & $6.428$ & $280$ \\
\Fastcat & $17$ & $6.071$ & $280$ \\
\regularnetselu & $14$ & $5.0$ & $280$ \\
\RF{} & $14$ & $5.0$ & $280$ \\
\XRF{} & $14$ & $5.0$ & $280$ \\
\XGBoost{} & $13$ & $4.642$ & $280$ \\
\mlrnetselu & $11$ & $3.928$ & $280$ \\
\lightgbm{} & $9$ & $3.214$ & $280$ \\
\regularnetstandard & $9$ & $3.214$ & $280$ \\
\regularnetbatchresblock & $8$ & $2.857$ & $280$ \\
\mlrnetfastselu & $8$ & $2.857$ & $280$ \\
\mlrnetstandard & $8$ & $2.857$ & $280$ \\
\Enet{} & $7$ & $2.5$ & $280$ \\
\mlrnetbatchresblock & $5$ & $1.785$ & $280$ \\
\regularnetfastselu & $5$ & $1.785$ & $280$ \\
\regularnetglu & $5$ & $1.785$ & $280$ \\
\LAS{} & $5$ & $1.785$ & $280$ \\
\Ridge{} & $4$ & $1.428$ & $280$ \\
\NuSVM{} & $4$ & $1.428$ & $280$ \\
\regularnetresblock & $4$ & $1.428$ & $280$ \\
\Kernel{} & $4$ & $1.428$ & $280$ \\
\mlrnetresblock & $3$ & $1.071$ & $280$ \\
\mlrnetfast & $3$ & $1.071$ & $280$ \\
\regularnetbatchstandard & $3$ & $1.071$ & $280$ \\
\regularnetfast & $2$ & $0.714$ & $280$ \\
\Adaboost{} & $2$ & $0.714$ & $280$ \\
\MARS{} & $2$ & $0.714$ & $280$ \\
\mlrnetbatchstandard & $1$ & $0.357$ & $280$ \\
\hline
\end{tabular}
\caption{method top1 count for \AUC{} and \Rscore{} with $n <= 1000$}
\end{table}

\begin{table}[h]
\centering
\footnotesize
\begin{tabular}{|l||c|c|c|}
\hline
method & \ERR{} and \RMSE{} & \%WIN & \# Datasets splits \\
\hline
\hline
\Catboost{} & $108$ & $24.54$ & $440$ \\
\XRF{} & $40$ & $9.090$ & $440$ \\
\Fastcat & $35$ & $7.954$ & $440$ \\
\XGBsklearn{} & $27$ & $6.136$ & $440$ \\
\RF{} & $25$ & $5.681$ & $440$ \\
\Adaboost{} & $23$ & $5.227$ & $440$ \\
\regularnetfastselu & $22$ & $5.0$ & $440$ \\
\regularnetselu & $19$ & $4.318$ & $440$ \\
\regularnetglu & $17$ & $3.863$ & $440$ \\
\lightgbm{} & $14$ & $3.181$ & $440$ \\
\XGBoost{} & $14$ & $3.181$ & $440$ \\
\Enet{} & $14$ & $3.181$ & $440$ \\
\regularnetbatchstandard & $13$ & $2.954$ & $440$ \\
\regularnetstandard & $11$ & $2.5$ & $440$ \\
\regularnetbatchresblock & $10$ & $2.272$ & $440$ \\
\LAS{} & $10$ & $2.272$ & $440$ \\
\regularnetresblock & $9$ & $2.045$ & $440$ \\
\regularnetfast & $7$ & $1.590$ & $440$ \\
\Kernel{} & $7$ & $1.590$ & $440$ \\
\NuSVM{} & $6$ & $1.363$ & $440$ \\
\MARS{} & $4$ & $0.909$ & $440$ \\
\CART{} & $4$ & $0.909$ & $440$ \\
\Ridge{} & $1$ & $0.227$ & $440$ \\
\hline
\end{tabular}
\caption{method top1 count excluding \trainmet{} for \ERR{} and \RMSE{}}
\end{table}

\begin{table}[h]
\centering
\footnotesize
\begin{tabular}{|l||c|c|c|}
\hline
method & \ERR{} and \RMSE{} & \%WIN & \# Datasets splits \\
\hline
\hline
\Catboost{} & $67$ & $23.92$ & $280$ \\
\Fastcat & $25$ & $8.928$ & $280$ \\
\Adaboost{} & $23$ & $8.214$ & $280$ \\
\regularnetselu & $17$ & $6.071$ & $280$ \\
\XRF{} & $14$ & $5.0$ & $280$ \\
\Enet{} & $14$ & $5.0$ & $280$ \\
\XGBsklearn{} & $14$ & $5.0$ & $280$ \\
\regularnetfastselu & $14$ & $5.0$ & $280$ \\
\RF{} & $12$ & $4.285$ & $280$ \\
\LAS{} & $10$ & $3.571$ & $280$ \\
\regularnetglu & $9$ & $3.214$ & $280$ \\
\XGBoost{} & $8$ & $2.857$ & $280$ \\
\regularnetstandard & $8$ & $2.857$ & $280$ \\
\lightgbm{} & $8$ & $2.857$ & $280$ \\
\regularnetfast & $7$ & $2.5$ & $280$ \\
\regularnetbatchresblock & $6$ & $2.142$ & $280$ \\
\NuSVM{} & $5$ & $1.785$ & $280$ \\
\CART{} & $4$ & $1.428$ & $280$ \\
\regularnetbatchstandard & $4$ & $1.428$ & $280$ \\
\MARS{} & $4$ & $1.428$ & $280$ \\
\Kernel{} & $4$ & $1.428$ & $280$ \\
\regularnetresblock & $3$ & $1.071$ & $280$ \\
\hline
\end{tabular}
\caption{method top1 count excluding \trainmet{} for \ERR{} and \RMSE{} with $n <= 1000$}
\end{table}

\begin{table}[h]
\centering
\footnotesize
\begin{tabular}{|l||c|c|c|}
\hline
method & \ERR{} and \RMSE{} & \%WIN & \# Datasets splits \\
\hline
\hline
\Catboost{} & $69$ & $27.93$ & $247$ \\
\Adaboost{} & $23$ & $9.311$ & $247$ \\
\XRF{} & $18$ & $7.287$ & $247$ \\
\Fastcat & $16$ & $6.477$ & $247$ \\
\regularnetselu & $15$ & $6.072$ & $247$ \\
\XGBoost{} & $12$ & $4.858$ & $247$ \\
\regularnetbatchstandard & $11$ & $4.453$ & $247$ \\
\RF{} & $11$ & $4.453$ & $247$ \\
\lightgbm{} & $10$ & $4.048$ & $247$ \\
\regularnetfastselu & $9$ & $3.643$ & $247$ \\
\Enet{} & $9$ & $3.643$ & $247$ \\
\XGBsklearn{} & $8$ & $3.238$ & $247$ \\
\regularnetglu & $7$ & $2.834$ & $247$ \\
\regularnetstandard & $7$ & $2.834$ & $247$ \\
\regularnetbatchresblock & $6$ & $2.429$ & $247$ \\
\regularnetfast & $5$ & $2.024$ & $247$ \\
\LAS{} & $5$ & $2.024$ & $247$ \\
\CART{} & $4$ & $1.619$ & $247$ \\
\regularnetresblock & $2$ & $0.809$ & $247$ \\
\hline
\end{tabular}
\caption{method top1 count excluding \trainmet{} for \ERR{} and \RMSE{} with min \ERR{} and \RMSE{} $<= 0.25$}
\end{table}

\begin{table}[h]
\centering
\footnotesize
\begin{tabular}{|l||c|c|c|}
\hline
method & \ERR{} and \RMSE{} & \%WIN & \# Datasets splits \\
\hline
\hline
\Catboost{} & $101$ & $22.95$ & $440$ \\
\XRF{} & $38$ & $8.636$ & $440$ \\
\Fastcat & $34$ & $7.727$ & $440$ \\
\mlrnetglu & $28$ & $6.363$ & $440$ \\
\XGBsklearn{} & $26$ & $5.909$ & $440$ \\
\RF{} & $24$ & $5.454$ & $440$ \\
\Adaboost{} & $23$ & $5.227$ & $440$ \\
\Enet{} & $14$ & $3.181$ & $440$ \\
\lightgbm{} & $14$ & $3.181$ & $440$ \\
\XGBoost{} & $13$ & $2.954$ & $440$ \\
\mlrnetselu & $12$ & $2.727$ & $440$ \\
\regularnetglu & $10$ & $2.272$ & $440$ \\
\regularnetfastselu & $10$ & $2.272$ & $440$ \\
\LAS{} & $10$ & $2.272$ & $440$ \\
\mlrnetfastselu & $10$ & $2.272$ & $440$ \\
\regularnetselu & $7$ & $1.590$ & $440$ \\
\regularnetresblock & $7$ & $1.590$ & $440$ \\
\mlrnetbatchresblock & $6$ & $1.363$ & $440$ \\
\regularnetstandard & $6$ & $1.363$ & $440$ \\
\Kernel{} & $6$ & $1.363$ & $440$ \\
\regularnetbatchstandard & $6$ & $1.363$ & $440$ \\
\mlrnetfast & $5$ & $1.136$ & $440$ \\
\NuSVM{} & $5$ & $1.136$ & $440$ \\
\mlrnetstandard & $5$ & $1.136$ & $440$ \\
\regularnetbatchresblock & $4$ & $0.909$ & $440$ \\
\CART{} & $4$ & $0.909$ & $440$ \\
\regularnetfast & $4$ & $0.909$ & $440$ \\
\mlrnetresblock & $3$ & $0.681$ & $440$ \\
\MARS{} & $2$ & $0.454$ & $440$ \\
\mlrnetbatchstandard & $2$ & $0.454$ & $440$ \\
\Ridge{} & $1$ & $0.227$ & $440$ \\
\hline
\end{tabular}
\caption{method top1 count for \ERR{} and \RMSE{}}
\end{table}

\begin{table}[h]
\centering
\footnotesize
\begin{tabular}{|l||c|c|c|}
\hline
method & \ERR{} and \RMSE{} & \%WIN & \# Datasets splits \\
\hline
\hline
\Catboost{} & $60$ & $21.42$ & $280$ \\
\Fastcat & $24$ & $8.571$ & $280$ \\
\Adaboost{} & $23$ & $8.214$ & $280$ \\
\mlrnetglu & $16$ & $5.714$ & $280$ \\
\Enet{} & $14$ & $5.0$ & $280$ \\
\XGBsklearn{} & $13$ & $4.642$ & $280$ \\
\XRF{} & $12$ & $4.285$ & $280$ \\
\mlrnetselu & $11$ & $3.928$ & $280$ \\
\RF{} & $11$ & $3.928$ & $280$ \\
\LAS{} & $10$ & $3.571$ & $280$ \\
\mlrnetfastselu & $9$ & $3.214$ & $280$ \\
\lightgbm{} & $8$ & $2.857$ & $280$ \\
\XGBoost{} & $7$ & $2.5$ & $280$ \\
\regularnetselu & $6$ & $2.142$ & $280$ \\
\regularnetfastselu & $6$ & $2.142$ & $280$ \\
\regularnetstandard & $5$ & $1.785$ & $280$ \\
\mlrnetbatchresblock & $5$ & $1.785$ & $280$ \\
\CART{} & $4$ & $1.428$ & $280$ \\
\regularnetglu & $4$ & $1.428$ & $280$ \\
\Kernel{} & $4$ & $1.428$ & $280$ \\
\regularnetfast & $4$ & $1.428$ & $280$ \\
\NuSVM{} & $4$ & $1.428$ & $280$ \\
\regularnetbatchresblock & $4$ & $1.428$ & $280$ \\
\regularnetbatchstandard & $3$ & $1.071$ & $280$ \\
\regularnetresblock & $3$ & $1.071$ & $280$ \\
\mlrnetstandard & $3$ & $1.071$ & $280$ \\
\mlrnetbatchstandard & $2$ & $0.714$ & $280$ \\
\MARS{} & $2$ & $0.714$ & $280$ \\
\mlrnetfast & $2$ & $0.714$ & $280$ \\
\mlrnetresblock & $1$ & $0.357$ & $280$ \\
\hline
\end{tabular}
\caption{method top1 count for \ERR{} and \RMSE{} with $n <= 1000$}
\end{table}

\begin{table}[h]
\centering
\footnotesize
\begin{tabular}{|l||c|c|c|}
\hline
method & \ERR{} and \RMSE{} & \%WIN & \# Datasets splits \\
\hline
\hline
\Catboost{} & $63$ & $25.30$ & $249$ \\
\mlrnetglu & $25$ & $10.04$ & $249$ \\
\Adaboost{} & $23$ & $9.236$ & $249$ \\
\XRF{} & $16$ & $6.425$ & $249$ \\
\Fastcat & $15$ & $6.024$ & $249$ \\
\RF{} & $11$ & $4.417$ & $249$ \\
\XGBoost{} & $11$ & $4.417$ & $249$ \\
\lightgbm{} & $10$ & $4.016$ & $249$ \\
\Enet{} & $9$ & $3.614$ & $249$ \\
\mlrnetselu & $8$ & $3.212$ & $249$ \\
\XGBsklearn{} & $7$ & $2.811$ & $249$ \\
\regularnetselu & $5$ & $2.008$ & $249$ \\
\LAS{} & $5$ & $2.008$ & $249$ \\
\mlrnetfastselu & $5$ & $2.008$ & $249$ \\
\regularnetstandard & $4$ & $1.606$ & $249$ \\
\regularnetbatchstandard & $4$ & $1.606$ & $249$ \\
\CART{} & $4$ & $1.606$ & $249$ \\
\mlrnetstandard & $3$ & $1.204$ & $249$ \\
\mlrnetbatchresblock & $3$ & $1.204$ & $249$ \\
\regularnetfast & $3$ & $1.204$ & $249$ \\
\regularnetfastselu & $3$ & $1.204$ & $249$ \\
\regularnetglu & $3$ & $1.204$ & $249$ \\
\regularnetresblock & $2$ & $0.803$ & $249$ \\
\mlrnetfast & $2$ & $0.803$ & $249$ \\
\mlrnetbatchstandard & $2$ & $0.803$ & $249$ \\
\regularnetbatchresblock & $2$ & $0.803$ & $249$ \\
\mlrnetresblock & $1$ & $0.401$ & $249$ \\
\hline
\end{tabular}
\caption{method top1 count for \ERR{} and \RMSE{} with min \ERR{} and \RMSE{} $<= 0.25$}
\end{table}

\begin{table}[h]
\centering
\footnotesize
\begin{tabular}{|l||c|c|c|}
\hline
method & \Rscore{} & \%WIN & \# Datasets splits \\
\hline
\hline
\Catboost{} & $52$ & $20.0$ & $260$ \\
\XRF{} & $33$ & $12.69$ & $260$ \\
\XGBsklearn{} & $20$ & $7.692$ & $260$ \\
\regularnetselu & $19$ & $7.307$ & $260$ \\
\regularnetfastselu & $19$ & $7.307$ & $260$ \\
\Fastcat & $17$ & $6.538$ & $260$ \\
\regularnetglu & $16$ & $6.153$ & $260$ \\
\RF{} & $14$ & $5.384$ & $260$ \\
\regularnetstandard & $9$ & $3.461$ & $260$ \\
\regularnetresblock & $8$ & $3.076$ & $260$ \\
\regularnetbatchstandard & $8$ & $3.076$ & $260$ \\
\Kernel{} & $7$ & $2.692$ & $260$ \\
\regularnetbatchresblock & $6$ & $2.307$ & $260$ \\
\NuSVM{} & $6$ & $2.307$ & $260$ \\
\LAS{} & $5$ & $1.923$ & $260$ \\
\Enet{} & $5$ & $1.923$ & $260$ \\
\MARS{} & $4$ & $1.538$ & $260$ \\
\lightgbm{} & $4$ & $1.538$ & $260$ \\
\XGBoost{} & $4$ & $1.538$ & $260$ \\
\regularnetfast & $3$ & $1.153$ & $260$ \\
\Ridge{} & $1$ & $0.384$ & $260$ \\
\hline
\end{tabular}
\caption{method top1 count excluding \trainmet{} for \Rscore{}}
\end{table}

\begin{table}[h]
\centering
\footnotesize
\begin{tabular}{|l||c|c|c|}
\hline
method & \Rscore{} & \%WIN & \# Datasets splits \\
\hline
\hline
\Catboost{} & $44$ & $29.33$ & $150$ \\
\regularnetselu & $17$ & $11.33$ & $150$ \\
\regularnetfastselu & $11$ & $7.333$ & $150$ \\
\XRF{} & $9$ & $6.0$ & $150$ \\
\XGBsklearn{} & $9$ & $6.0$ & $150$ \\
\regularnetglu & $8$ & $5.333$ & $150$ \\
\Fastcat & $7$ & $4.666$ & $150$ \\
\regularnetstandard & $6$ & $4.0$ & $150$ \\
\RF{} & $5$ & $3.333$ & $150$ \\
\NuSVM{} & $5$ & $3.333$ & $150$ \\
\LAS{} & $5$ & $3.333$ & $150$ \\
\Enet{} & $5$ & $3.333$ & $150$ \\
\MARS{} & $4$ & $2.666$ & $150$ \\
\Kernel{} & $4$ & $2.666$ & $150$ \\
\XGBoost{} & $4$ & $2.666$ & $150$ \\
\regularnetfast & $3$ & $2.0$ & $150$ \\
\regularnetbatchresblock & $2$ & $1.333$ & $150$ \\
\regularnetresblock & $2$ & $1.333$ & $150$ \\
\hline
\end{tabular}
\caption{method top1 count excluding \trainmet{} for \Rscore{} with $n <= 1000$}
\end{table}

\begin{table}[h]
\centering
\footnotesize
\begin{tabular}{|l||c|c|c|}
\hline
method & \Rscore{} & \%WIN & \# Datasets splits \\
\hline
\hline
\Catboost{} & $47$ & $18.07$ & $260$ \\
\XRF{} & $33$ & $12.69$ & $260$ \\
\mlrnetglu & $26$ & $10.0$ & $260$ \\
\XGBsklearn{} & $19$ & $7.307$ & $260$ \\
\Fastcat & $17$ & $6.538$ & $260$ \\
\RF{} & $13$ & $5.0$ & $260$ \\
\mlrnetselu & $10$ & $3.846$ & $260$ \\
\regularnetglu & $9$ & $3.461$ & $260$ \\
\regularnetfastselu & $9$ & $3.461$ & $260$ \\
\mlrnetfastselu & $8$ & $3.076$ & $260$ \\
\regularnetselu & $7$ & $2.692$ & $260$ \\
\Kernel{} & $6$ & $2.307$ & $260$ \\
\regularnetresblock & $6$ & $2.307$ & $260$ \\
\Enet{} & $5$ & $1.923$ & $260$ \\
\LAS{} & $5$ & $1.923$ & $260$ \\
\NuSVM{} & $5$ & $1.923$ & $260$ \\
\mlrnetresblock & $4$ & $1.538$ & $260$ \\
\lightgbm{} & $4$ & $1.538$ & $260$ \\
\mlrnetfast & $4$ & $1.538$ & $260$ \\
\XGBoost{} & $4$ & $1.538$ & $260$ \\
\regularnetstandard & $4$ & $1.538$ & $260$ \\
\mlrnetstandard & $4$ & $1.538$ & $260$ \\
\mlrnetbatchresblock & $3$ & $1.153$ & $260$ \\
\MARS{} & $2$ & $0.769$ & $260$ \\
\regularnetbatchresblock & $2$ & $0.769$ & $260$ \\
\regularnetbatchstandard & $2$ & $0.769$ & $260$ \\
\Ridge{} & $1$ & $0.384$ & $260$ \\
\regularnetfast & $1$ & $0.384$ & $260$ \\
\hline
\end{tabular}
\caption{method top1 count for \Rscore{}}
\end{table}

\begin{table}[h]
\centering
\footnotesize
\begin{tabular}{|l||c|c|c|}
\hline
method & \Rscore{} & \%WIN & \# Datasets splits \\
\hline
\hline
\Catboost{} & $39$ & $26.0$ & $150$ \\
\mlrnetglu & $14$ & $9.333$ & $150$ \\
\mlrnetselu & $9$ & $6.0$ & $150$ \\
\XRF{} & $9$ & $6.0$ & $150$ \\
\XGBsklearn{} & $8$ & $5.333$ & $150$ \\
\mlrnetfastselu & $7$ & $4.666$ & $150$ \\
\Fastcat & $7$ & $4.666$ & $150$ \\
\regularnetselu & $6$ & $4.0$ & $150$ \\
\regularnetfastselu & $5$ & $3.333$ & $150$ \\
\Enet{} & $5$ & $3.333$ & $150$ \\
\LAS{} & $5$ & $3.333$ & $150$ \\
\RF{} & $4$ & $2.666$ & $150$ \\
\Kernel{} & $4$ & $2.666$ & $150$ \\
\NuSVM{} & $4$ & $2.666$ & $150$ \\
\XGBoost{} & $4$ & $2.666$ & $150$ \\
\regularnetglu & $3$ & $2.0$ & $150$ \\
\regularnetstandard & $3$ & $2.0$ & $150$ \\
\mlrnetbatchresblock & $2$ & $1.333$ & $150$ \\
\MARS{} & $2$ & $1.333$ & $150$ \\
\regularnetresblock & $2$ & $1.333$ & $150$ \\
\mlrnetresblock & $2$ & $1.333$ & $150$ \\
\regularnetbatchresblock & $2$ & $1.333$ & $150$ \\
\mlrnetstandard & $2$ & $1.333$ & $150$ \\
\regularnetfast & $1$ & $0.666$ & $150$ \\
\mlrnetfast & $1$ & $0.666$ & $150$ \\
\hline
\end{tabular}
\caption{method top1 count for \Rscore{} with $n <= 1000$}
\end{table}

\begin{table}[h]
\centering
\footnotesize
\begin{tabular}{|l||c|c|c|}
\hline
method & \RMSE{} & \%WIN & \# Datasets splits \\
\hline
\hline
\Catboost{} & $52$ & $20.0$ & $260$ \\
\XRF{} & $33$ & $12.69$ & $260$ \\
\XGBsklearn{} & $20$ & $7.692$ & $260$ \\
\regularnetselu & $19$ & $7.307$ & $260$ \\
\regularnetfastselu & $19$ & $7.307$ & $260$ \\
\Fastcat & $17$ & $6.538$ & $260$ \\
\regularnetglu & $16$ & $6.153$ & $260$ \\
\RF{} & $14$ & $5.384$ & $260$ \\
\regularnetstandard & $9$ & $3.461$ & $260$ \\
\regularnetresblock & $8$ & $3.076$ & $260$ \\
\regularnetbatchstandard & $8$ & $3.076$ & $260$ \\
\Kernel{} & $7$ & $2.692$ & $260$ \\
\regularnetbatchresblock & $6$ & $2.307$ & $260$ \\
\NuSVM{} & $6$ & $2.307$ & $260$ \\
\LAS{} & $5$ & $1.923$ & $260$ \\
\Enet{} & $5$ & $1.923$ & $260$ \\
\MARS{} & $4$ & $1.538$ & $260$ \\
\lightgbm{} & $4$ & $1.538$ & $260$ \\
\XGBoost{} & $4$ & $1.538$ & $260$ \\
\regularnetfast & $3$ & $1.153$ & $260$ \\
\Ridge{} & $1$ & $0.384$ & $260$ \\
\hline
\end{tabular}
\caption{method top1 count excluding \trainmet{} for \RMSE{}}
\end{table}

\begin{table}[h]
\centering
\footnotesize
\begin{tabular}{|l||c|c|c|}
\hline
method & \RMSE{} & \%WIN & \# Datasets splits \\
\hline
\hline
\Catboost{} & $44$ & $29.33$ & $150$ \\
\regularnetselu & $17$ & $11.33$ & $150$ \\
\regularnetfastselu & $11$ & $7.333$ & $150$ \\
\XRF{} & $9$ & $6.0$ & $150$ \\
\XGBsklearn{} & $9$ & $6.0$ & $150$ \\
\regularnetglu & $8$ & $5.333$ & $150$ \\
\Fastcat & $7$ & $4.666$ & $150$ \\
\regularnetstandard & $6$ & $4.0$ & $150$ \\
\RF{} & $5$ & $3.333$ & $150$ \\
\NuSVM{} & $5$ & $3.333$ & $150$ \\
\LAS{} & $5$ & $3.333$ & $150$ \\
\Enet{} & $5$ & $3.333$ & $150$ \\
\MARS{} & $4$ & $2.666$ & $150$ \\
\Kernel{} & $4$ & $2.666$ & $150$ \\
\XGBoost{} & $4$ & $2.666$ & $150$ \\
\regularnetfast & $3$ & $2.0$ & $150$ \\
\regularnetbatchresblock & $2$ & $1.333$ & $150$ \\
\regularnetresblock & $2$ & $1.333$ & $150$ \\
\hline
\end{tabular}
\caption{method top1 count excluding \trainmet{} for \RMSE{} with $n <= 1000$}
\end{table}

\begin{table}[h]
\centering
\footnotesize
\begin{tabular}{|l||c|c|c|}
\hline
method & \RMSE{} & \%WIN & \# Datasets splits \\
\hline
\hline
\Catboost{} & $20$ & $25.0$ & $80$ \\
\regularnetselu & $15$ & $18.75$ & $80$ \\
\XRF{} & $12$ & $15.0$ & $80$ \\
\regularnetbatchstandard & $7$ & $8.75$ & $80$ \\
\regularnetfastselu & $6$ & $7.5$ & $80$ \\
\regularnetglu & $6$ & $7.5$ & $80$ \\
\regularnetstandard & $5$ & $6.25$ & $80$ \\
\regularnetbatchresblock & $3$ & $3.75$ & $80$ \\
\XGBoost{} & $2$ & $2.5$ & $80$ \\
\XGBsklearn{} & $2$ & $2.5$ & $80$ \\
\regularnetfast & $1$ & $1.25$ & $80$ \\
\regularnetresblock & $1$ & $1.25$ & $80$ \\
\hline
\end{tabular}
\caption{method top1 count excluding \trainmet{} for \RMSE{} with min \RMSE{} $<= 0.25$}
\end{table}

\begin{table}[h]
\centering
\footnotesize
\begin{tabular}{|l||c|c|c|}
\hline
method & \RMSE{} & \%WIN & \# Datasets splits \\
\hline
\hline
\Catboost{} & $47$ & $18.07$ & $260$ \\
\XRF{} & $33$ & $12.69$ & $260$ \\
\mlrnetglu & $26$ & $10.0$ & $260$ \\
\XGBsklearn{} & $19$ & $7.307$ & $260$ \\
\Fastcat & $17$ & $6.538$ & $260$ \\
\RF{} & $13$ & $5.0$ & $260$ \\
\mlrnetselu & $10$ & $3.846$ & $260$ \\
\regularnetglu & $9$ & $3.461$ & $260$ \\
\regularnetfastselu & $9$ & $3.461$ & $260$ \\
\mlrnetfastselu & $8$ & $3.076$ & $260$ \\
\regularnetselu & $7$ & $2.692$ & $260$ \\
\regularnetresblock & $6$ & $2.307$ & $260$ \\
\Kernel{} & $6$ & $2.307$ & $260$ \\
\LAS{} & $5$ & $1.923$ & $260$ \\
\Enet{} & $5$ & $1.923$ & $260$ \\
\NuSVM{} & $5$ & $1.923$ & $260$ \\
\mlrnetfast & $4$ & $1.538$ & $260$ \\
\mlrnetstandard & $4$ & $1.538$ & $260$ \\
\regularnetstandard & $4$ & $1.538$ & $260$ \\
\mlrnetbatchresblock & $4$ & $1.538$ & $260$ \\
\XGBoost{} & $4$ & $1.538$ & $260$ \\
\lightgbm{} & $4$ & $1.538$ & $260$ \\
\mlrnetresblock & $3$ & $1.153$ & $260$ \\
\MARS{} & $2$ & $0.769$ & $260$ \\
\regularnetbatchresblock & $2$ & $0.769$ & $260$ \\
\regularnetbatchstandard & $2$ & $0.769$ & $260$ \\
\Ridge{} & $1$ & $0.384$ & $260$ \\
\regularnetfast & $1$ & $0.384$ & $260$ \\
\hline
\end{tabular}
\caption{method top1 count for \RMSE{}}
\end{table}

\begin{table}[h]
\centering
\footnotesize
\begin{tabular}{|l||c|c|c|}
\hline
method & \RMSE{} & \%WIN & \# Datasets splits \\
\hline
\hline
\Catboost{} & $39$ & $26.0$ & $150$ \\
\mlrnetglu & $14$ & $9.333$ & $150$ \\
\mlrnetselu & $9$ & $6.0$ & $150$ \\
\XRF{} & $9$ & $6.0$ & $150$ \\
\XGBsklearn{} & $8$ & $5.333$ & $150$ \\
\mlrnetfastselu & $7$ & $4.666$ & $150$ \\
\Fastcat & $7$ & $4.666$ & $150$ \\
\regularnetselu & $6$ & $4.0$ & $150$ \\
\regularnetfastselu & $5$ & $3.333$ & $150$ \\
\Enet{} & $5$ & $3.333$ & $150$ \\
\LAS{} & $5$ & $3.333$ & $150$ \\
\RF{} & $4$ & $2.666$ & $150$ \\
\Kernel{} & $4$ & $2.666$ & $150$ \\
\NuSVM{} & $4$ & $2.666$ & $150$ \\
\XGBoost{} & $4$ & $2.666$ & $150$ \\
\regularnetglu & $3$ & $2.0$ & $150$ \\
\mlrnetbatchresblock & $3$ & $2.0$ & $150$ \\
\regularnetstandard & $3$ & $2.0$ & $150$ \\
\MARS{} & $2$ & $1.333$ & $150$ \\
\regularnetresblock & $2$ & $1.333$ & $150$ \\
\regularnetbatchresblock & $2$ & $1.333$ & $150$ \\
\mlrnetstandard & $2$ & $1.333$ & $150$ \\
\mlrnetfast & $1$ & $0.666$ & $150$ \\
\regularnetfast & $1$ & $0.666$ & $150$ \\
\mlrnetresblock & $1$ & $0.666$ & $150$ \\
\hline
\end{tabular}
\caption{method top1 count for \RMSE{} with $n <= 1000$}
\end{table}

\begin{table}[h]
\centering
\footnotesize
\begin{tabular}{|l||c|c|c|}
\hline
method & \RMSE{} & \%WIN & \# Datasets splits \\
\hline
\hline
\mlrnetglu & $23$ & $28.39$ & $81$ \\
\Catboost{} & $16$ & $19.75$ & $81$ \\
\XRF{} & $12$ & $14.81$ & $81$ \\
\mlrnetselu & $6$ & $7.407$ & $81$ \\
\regularnetselu & $5$ & $6.172$ & $81$ \\
\mlrnetfastselu & $3$ & $3.703$ & $81$ \\
\regularnetfastselu & $2$ & $2.469$ & $81$ \\
\regularnetglu & $2$ & $2.469$ & $81$ \\
\mlrnetstandard & $2$ & $2.469$ & $81$ \\
\regularnetstandard & $2$ & $2.469$ & $81$ \\
\XGBoost{} & $2$ & $2.469$ & $81$ \\
\mlrnetbatchresblock & $1$ & $1.234$ & $81$ \\
\regularnetbatchstandard & $1$ & $1.234$ & $81$ \\
\mlrnetresblock & $1$ & $1.234$ & $81$ \\
\regularnetresblock & $1$ & $1.234$ & $81$ \\
\mlrnetfast & $1$ & $1.234$ & $81$ \\
\XGBsklearn{} & $1$ & $1.234$ & $81$ \\
\hline
\end{tabular}
\caption{method top1 count for \RMSE{} with min \RMSE{} $<= 0.25$}
\end{table}

\begin{table}[h]
\centering
\footnotesize
\begin{tabular}{|l||c|c|c|}
\hline
method & \AUC{} & \%WIN & \# Datasets splits \\
\hline
\hline
\Catboost{} & $49$ & $27.22$ & $180$ \\
\XGBsklearn{} & $18$ & $10.0$ & $180$ \\
\XGBoost{} & $17$ & $9.444$ & $180$ \\
\RF{} & $15$ & $8.333$ & $180$ \\
\lightgbm{} & $11$ & $6.111$ & $180$ \\
\Fastcat & $10$ & $5.555$ & $180$ \\
\XRF{} & $10$ & $5.555$ & $180$ \\
\regularnetselu & $10$ & $5.555$ & $180$ \\
\regularnetstandard & $7$ & $3.888$ & $180$ \\
\regularnetbatchresblock & $6$ & $3.333$ & $180$ \\
\Ridge{} & $5$ & $2.777$ & $180$ \\
\regularnetbatchstandard & $4$ & $2.222$ & $180$ \\
\regularnetglu & $4$ & $2.222$ & $180$ \\
\regularnetresblock & $3$ & $1.666$ & $180$ \\
\Adaboost{} & $3$ & $1.666$ & $180$ \\
\LAS{} & $2$ & $1.111$ & $180$ \\
\regularnetfast & $2$ & $1.111$ & $180$ \\
\regularnetfastselu & $2$ & $1.111$ & $180$ \\
\Enet{} & $2$ & $1.111$ & $180$ \\
\hline
\end{tabular}
\caption{method top1 count excluding \trainmet{} for \AUC{}}
\end{table}

\begin{table}[h]
\centering
\footnotesize
\begin{tabular}{|l||c|c|c|}
\hline
method & \AUC{} & \%WIN & \# Datasets splits \\
\hline
\hline
\XGBsklearn{} & $18$ & $13.84$ & $130$ \\
\Catboost{} & $15$ & $11.53$ & $130$ \\
\RF{} & $11$ & $8.461$ & $130$ \\
\Fastcat & $10$ & $7.692$ & $130$ \\
\lightgbm{} & $10$ & $7.692$ & $130$ \\
\XGBoost{} & $10$ & $7.692$ & $130$ \\
\regularnetselu & $9$ & $6.923$ & $130$ \\
\XRF{} & $7$ & $5.384$ & $130$ \\
\regularnetstandard & $7$ & $5.384$ & $130$ \\
\regularnetbatchresblock & $6$ & $4.615$ & $130$ \\
\Ridge{} & $5$ & $3.846$ & $130$ \\
\regularnetbatchstandard & $4$ & $3.076$ & $130$ \\
\regularnetglu & $4$ & $3.076$ & $130$ \\
\regularnetresblock & $3$ & $2.307$ & $130$ \\
\Adaboost{} & $3$ & $2.307$ & $130$ \\
\regularnetfastselu & $2$ & $1.538$ & $130$ \\
\regularnetfast & $2$ & $1.538$ & $130$ \\
\LAS{} & $2$ & $1.538$ & $130$ \\
\Enet{} & $2$ & $1.538$ & $130$ \\
\hline
\end{tabular}
\caption{method top1 count excluding \trainmet{} for \AUC{} with $n <= 1000$}
\end{table}

\begin{table}[h]
\centering
\footnotesize
\begin{tabular}{|l||c|c|c|}
\hline
method & \AUC{} & \%WIN & \# Datasets splits \\
\hline
\hline
\Catboost{} & $47$ & $26.11$ & $180$ \\
\XGBsklearn{} & $18$ & $10.0$ & $180$ \\
\XGBoost{} & $16$ & $8.888$ & $180$ \\
\RF{} & $14$ & $7.777$ & $180$ \\
\Fastcat & $10$ & $5.555$ & $180$ \\
\lightgbm{} & $10$ & $5.555$ & $180$ \\
\regularnetselu & $9$ & $5.0$ & $180$ \\
\XRF{} & $8$ & $4.444$ & $180$ \\
\regularnetbatchresblock & $6$ & $3.333$ & $180$ \\
\mlrnetstandard & $6$ & $3.333$ & $180$ \\
\regularnetstandard & $6$ & $3.333$ & $180$ \\
\mlrnetglu & $4$ & $2.222$ & $180$ \\
\Ridge{} & $4$ & $2.222$ & $180$ \\
\regularnetbatchstandard & $3$ & $1.666$ & $180$ \\
\mlrnetbatchresblock & $3$ & $1.666$ & $180$ \\
\Enet{} & $2$ & $1.111$ & $180$ \\
\Adaboost{} & $2$ & $1.111$ & $180$ \\
\mlrnetfast & $2$ & $1.111$ & $180$ \\
\mlrnetselu & $2$ & $1.111$ & $180$ \\
\regularnetglu & $2$ & $1.111$ & $180$ \\
\regularnetresblock & $2$ & $1.111$ & $180$ \\
\regularnetfast & $1$ & $0.555$ & $180$ \\
\mlrnetbatchstandard & $1$ & $0.555$ & $180$ \\
\mlrnetresblock & $1$ & $0.555$ & $180$ \\
\mlrnetfastselu & $1$ & $0.555$ & $180$ \\
\hline
\end{tabular}
\caption{method top1 count for \AUC{}}
\end{table}

\begin{table}[h]
\centering
\footnotesize
\begin{tabular}{|l||c|c|c|}
\hline
method & \AUC{} & \%WIN & \# Datasets splits \\
\hline
\hline
\XGBsklearn{} & $18$ & $13.84$ & $130$ \\
\Catboost{} & $13$ & $10.0$ & $130$ \\
\Fastcat & $10$ & $7.692$ & $130$ \\
\RF{} & $10$ & $7.692$ & $130$ \\
\lightgbm{} & $9$ & $6.923$ & $130$ \\
\XGBoost{} & $9$ & $6.923$ & $130$ \\
\regularnetselu & $8$ & $6.153$ & $130$ \\
\regularnetbatchresblock & $6$ & $4.615$ & $130$ \\
\mlrnetstandard & $6$ & $4.615$ & $130$ \\
\regularnetstandard & $6$ & $4.615$ & $130$ \\
\XRF{} & $5$ & $3.846$ & $130$ \\
\mlrnetglu & $4$ & $3.076$ & $130$ \\
\Ridge{} & $4$ & $3.076$ & $130$ \\
\regularnetbatchstandard & $3$ & $2.307$ & $130$ \\
\mlrnetbatchresblock & $3$ & $2.307$ & $130$ \\
\Enet{} & $2$ & $1.538$ & $130$ \\
\Adaboost{} & $2$ & $1.538$ & $130$ \\
\mlrnetfast & $2$ & $1.538$ & $130$ \\
\mlrnetselu & $2$ & $1.538$ & $130$ \\
\regularnetglu & $2$ & $1.538$ & $130$ \\
\regularnetresblock & $2$ & $1.538$ & $130$ \\
\regularnetfast & $1$ & $0.769$ & $130$ \\
\mlrnetbatchstandard & $1$ & $0.769$ & $130$ \\
\mlrnetresblock & $1$ & $0.769$ & $130$ \\
\mlrnetfastselu & $1$ & $0.769$ & $130$ \\
\hline
\end{tabular}
\caption{method top1 count for \AUC{} with $n <= 1000$}
\end{table}

\begin{table}[h]
\centering
\footnotesize
\begin{tabular}{|l||c|c|c|}
\hline
method & \ERR{} & \%WIN & \# Datasets splits \\
\hline
\hline
\Catboost{} & $56$ & $31.11$ & $180$ \\
\Adaboost{} & $23$ & $12.77$ & $180$ \\
\Fastcat & $18$ & $10.0$ & $180$ \\
\RF{} & $11$ & $6.111$ & $180$ \\
\lightgbm{} & $10$ & $5.555$ & $180$ \\
\XGBoost{} & $10$ & $5.555$ & $180$ \\
\Enet{} & $9$ & $5.0$ & $180$ \\
\XRF{} & $7$ & $3.888$ & $180$ \\
\XGBsklearn{} & $7$ & $3.888$ & $180$ \\
\regularnetbatchstandard & $5$ & $2.777$ & $180$ \\
\LAS{} & $5$ & $2.777$ & $180$ \\
\regularnetbatchresblock & $4$ & $2.222$ & $180$ \\
\regularnetfast & $4$ & $2.222$ & $180$ \\
\CART{} & $4$ & $2.222$ & $180$ \\
\regularnetfastselu & $3$ & $1.666$ & $180$ \\
\regularnetstandard & $2$ & $1.111$ & $180$ \\
\regularnetglu & $1$ & $0.555$ & $180$ \\
\regularnetresblock & $1$ & $0.555$ & $180$ \\
\hline
\end{tabular}
\caption{method top1 count excluding \trainmet{} for \ERR{}}
\end{table}

\begin{table}[h]
\centering
\footnotesize
\begin{tabular}{|l||c|c|c|}
\hline
method & \ERR{} & \%WIN & \# Datasets splits \\
\hline
\hline
\Adaboost{} & $23$ & $17.69$ & $130$ \\
\Catboost{} & $23$ & $17.69$ & $130$ \\
\Fastcat & $18$ & $13.84$ & $130$ \\
\Enet{} & $9$ & $6.923$ & $130$ \\
\lightgbm{} & $8$ & $6.153$ & $130$ \\
\RF{} & $7$ & $5.384$ & $130$ \\
\LAS{} & $5$ & $3.846$ & $130$ \\
\XRF{} & $5$ & $3.846$ & $130$ \\
\XGBsklearn{} & $5$ & $3.846$ & $130$ \\
\regularnetbatchresblock & $4$ & $3.076$ & $130$ \\
\regularnetbatchstandard & $4$ & $3.076$ & $130$ \\
\regularnetfast & $4$ & $3.076$ & $130$ \\
\CART{} & $4$ & $3.076$ & $130$ \\
\XGBoost{} & $4$ & $3.076$ & $130$ \\
\regularnetfastselu & $3$ & $2.307$ & $130$ \\
\regularnetstandard & $2$ & $1.538$ & $130$ \\
\regularnetglu & $1$ & $0.769$ & $130$ \\
\regularnetresblock & $1$ & $0.769$ & $130$ \\
\hline
\end{tabular}
\caption{method top1 count excluding \trainmet{} for \ERR{} with $n <= 1000$}
\end{table}

\begin{table}[h]
\centering
\footnotesize
\begin{tabular}{|l||c|c|c|}
\hline
method & \ERR{} & \%WIN & \# Datasets splits \\
\hline
\hline
\Catboost{} & $49$ & $29.34$ & $167$ \\
\Adaboost{} & $23$ & $13.77$ & $167$ \\
\Fastcat & $16$ & $9.580$ & $167$ \\
\RF{} & $11$ & $6.586$ & $167$ \\
\lightgbm{} & $10$ & $5.988$ & $167$ \\
\XGBoost{} & $10$ & $5.988$ & $167$ \\
\Enet{} & $9$ & $5.389$ & $167$ \\
\XRF{} & $6$ & $3.592$ & $167$ \\
\XGBsklearn{} & $6$ & $3.592$ & $167$ \\
\LAS{} & $5$ & $2.994$ & $167$ \\
\regularnetbatchstandard & $4$ & $2.395$ & $167$ \\
\regularnetfast & $4$ & $2.395$ & $167$ \\
\CART{} & $4$ & $2.395$ & $167$ \\
\regularnetbatchresblock & $3$ & $1.796$ & $167$ \\
\regularnetfastselu & $3$ & $1.796$ & $167$ \\
\regularnetstandard & $2$ & $1.197$ & $167$ \\
\regularnetglu & $1$ & $0.598$ & $167$ \\
\regularnetresblock & $1$ & $0.598$ & $167$ \\
\hline
\end{tabular}
\caption{method top1 count excluding \trainmet{} for \ERR{} with min \ERR{} $<= 0.25$}
\end{table}

\begin{table}[h]
\centering
\footnotesize
\begin{tabular}{|l||c|c|c|}
\hline
method & \ERR{} & \%WIN & \# Datasets splits \\
\hline
\hline
\Catboost{} & $54$ & $30.0$ & $180$ \\
\Adaboost{} & $23$ & $12.77$ & $180$ \\
\Fastcat & $17$ & $9.444$ & $180$ \\
\RF{} & $11$ & $6.111$ & $180$ \\
\lightgbm{} & $10$ & $5.555$ & $180$ \\
\XGBoost{} & $9$ & $5.0$ & $180$ \\
\Enet{} & $9$ & $5.0$ & $180$ \\
\XGBsklearn{} & $7$ & $3.888$ & $180$ \\
\XRF{} & $5$ & $2.777$ & $180$ \\
\LAS{} & $5$ & $2.777$ & $180$ \\
\CART{} & $4$ & $2.222$ & $180$ \\
\regularnetbatchstandard & $4$ & $2.222$ & $180$ \\
\regularnetfast & $3$ & $1.666$ & $180$ \\
\regularnetbatchresblock & $2$ & $1.111$ & $180$ \\
\mlrnetglu & $2$ & $1.111$ & $180$ \\
\mlrnetfastselu & $2$ & $1.111$ & $180$ \\
\regularnetstandard & $2$ & $1.111$ & $180$ \\
\mlrnetbatchstandard & $2$ & $1.111$ & $180$ \\
\mlrnetbatchresblock & $2$ & $1.111$ & $180$ \\
\mlrnetselu & $2$ & $1.111$ & $180$ \\
\regularnetfastselu & $1$ & $0.555$ & $180$ \\
\regularnetresblock & $1$ & $0.555$ & $180$ \\
\mlrnetstandard & $1$ & $0.555$ & $180$ \\
\regularnetglu & $1$ & $0.555$ & $180$ \\
\mlrnetfast & $1$ & $0.555$ & $180$ \\
\hline
\end{tabular}
\caption{method top1 count for \ERR{}}
\end{table}

\begin{table}[h]
\centering
\footnotesize
\begin{tabular}{|l||c|c|c|}
\hline
method & \ERR{} & \%WIN & \# Datasets splits \\
\hline
\hline
\Adaboost{} & $23$ & $17.69$ & $130$ \\
\Catboost{} & $21$ & $16.15$ & $130$ \\
\Fastcat & $17$ & $13.07$ & $130$ \\
\Enet{} & $9$ & $6.923$ & $130$ \\
\lightgbm{} & $8$ & $6.153$ & $130$ \\
\RF{} & $7$ & $5.384$ & $130$ \\
\LAS{} & $5$ & $3.846$ & $130$ \\
\XGBsklearn{} & $5$ & $3.846$ & $130$ \\
\CART{} & $4$ & $3.076$ & $130$ \\
\regularnetbatchstandard & $3$ & $2.307$ & $130$ \\
\XGBoost{} & $3$ & $2.307$ & $130$ \\
\XRF{} & $3$ & $2.307$ & $130$ \\
\regularnetfast & $3$ & $2.307$ & $130$ \\
\mlrnetglu & $2$ & $1.538$ & $130$ \\
\mlrnetfastselu & $2$ & $1.538$ & $130$ \\
\regularnetstandard & $2$ & $1.538$ & $130$ \\
\mlrnetbatchstandard & $2$ & $1.538$ & $130$ \\
\mlrnetbatchresblock & $2$ & $1.538$ & $130$ \\
\mlrnetselu & $2$ & $1.538$ & $130$ \\
\regularnetbatchresblock & $2$ & $1.538$ & $130$ \\
\regularnetfastselu & $1$ & $0.769$ & $130$ \\
\regularnetresblock & $1$ & $0.769$ & $130$ \\
\mlrnetstandard & $1$ & $0.769$ & $130$ \\
\regularnetglu & $1$ & $0.769$ & $130$ \\
\mlrnetfast & $1$ & $0.769$ & $130$ \\
\hline
\end{tabular}
\caption{method top1 count for \ERR{} with $n <= 1000$}
\end{table}

\begin{table}[h]
\centering
\footnotesize
\begin{tabular}{|l||c|c|c|}
\hline
method & \ERR{} & \%WIN & \# Datasets splits \\
\hline
\hline
\Catboost{} & $47$ & $27.97$ & $168$ \\
\Adaboost{} & $23$ & $13.69$ & $168$ \\
\Fastcat & $15$ & $8.928$ & $168$ \\
\RF{} & $11$ & $6.547$ & $168$ \\
\lightgbm{} & $10$ & $5.952$ & $168$ \\
\XGBoost{} & $9$ & $5.357$ & $168$ \\
\Enet{} & $9$ & $5.357$ & $168$ \\
\XGBsklearn{} & $6$ & $3.571$ & $168$ \\
\LAS{} & $5$ & $2.976$ & $168$ \\
\XRF{} & $4$ & $2.380$ & $168$ \\
\CART{} & $4$ & $2.380$ & $168$ \\
\regularnetbatchstandard & $3$ & $1.785$ & $168$ \\
\regularnetfast & $3$ & $1.785$ & $168$ \\
\regularnetbatchresblock & $2$ & $1.190$ & $168$ \\
\mlrnetglu & $2$ & $1.190$ & $168$ \\
\mlrnetfastselu & $2$ & $1.190$ & $168$ \\
\regularnetstandard & $2$ & $1.190$ & $168$ \\
\mlrnetbatchstandard & $2$ & $1.190$ & $168$ \\
\mlrnetbatchresblock & $2$ & $1.190$ & $168$ \\
\mlrnetselu & $2$ & $1.190$ & $168$ \\
\regularnetfastselu & $1$ & $0.595$ & $168$ \\
\regularnetresblock & $1$ & $0.595$ & $168$ \\
\mlrnetstandard & $1$ & $0.595$ & $168$ \\
\regularnetglu & $1$ & $0.595$ & $168$ \\
\mlrnetfast & $1$ & $0.595$ & $168$ \\
\hline
\end{tabular}
\caption{method top1 count for \ERR{} with min \ERR{} $<= 0.25$}
\end{table}
