# Supplementary material for: AdaCap: Adaptive Capacity control for Feed-Forward Neural Networks
Source: arXiv:2205.07860 source file (2022-05-09)
Supplement: Supplementary file 4 [file AppendixTableTop1CountVS.tex]

\clearpage

\begin{table}[h]
\centering
\footnotesize
% [inline block 0: 90 envs, 53608 chars -> data_tex | \begin{tabular}{|l||c|c|c|} \hline...]

\caption{\DNN{} vs \GBDT{} top1 count for \ERR{} with min \ERR{} $<= 0.25$}
\end{table}
